# Supplementary material for: Nanomechanical characterization of the Kondo charge dynamics in a carbon nanotube
Source: arXiv:1802.00522 ancillary file (2018-04-23)
Supplement: Supplementary file 1 [file supplement.pdf]

# Nanomechanical characterization of the Kondo charge dynamics in a carbon nanotube Supplementary Material

K. J. G. Götz, D. R. Schmid, F. J. Schupp, P. L. Stiller, Ch. Strunk, and A. K. Hüttel\*  
*Institute for Experimental and Applied Physics, University of Regensburg, Universitätsstr. 31, 93053 Regensburg, Germany*  
(Dated: April 23, 2018)

## CONTENTS

|                                                         |   |
|---------------------------------------------------------|---|
| I. Fabrication and device details                       | 1 |
| II. Capacitive sensitivity                              | 1 |
| III. Gate voltage dependence of the resonance frequency | 3 |
| IV. Comparison with Gerland et al. [1]                  | 4 |
| References                                              | 4 |

## I. FABRICATION AND DEVICE DETAILS

Both devices A and B have been fabricated in essentially the same way. On a highly p+ doped silicon wafer with a thermally dry-grown surface oxide, contact electrodes, leads, and bond pads are deposited via optical and electron beam lithography. Then the silicon oxide surface is anisotropically dry-etched to deepen the trenches between the electrodes. As last step, carbon nanotube growth catalyst is lithographically deposited at the center of the electrode structure, and chemical vapour deposition growth is performed [2]. The characteristic fabrication parameters of the two devices are summarized in Table S-I. Given that we do not image our devices after fabrication, the distance between the contacts provides an approximation for the active nanotube segment length.

Figure S-1 is a larger version of the characterization measurements already presented in Fig. 1(b,c) of the main text. The regularity of the transport spectrum and the transition from strong Coulomb blockade close to the electronic band gap to complex, Kondo-dominated behaviour at large positive gate voltage becomes immediately visible. Device B has in [4] also been characterized in the Fabry-Perot regime in hole conduction, resulting in an electronic length of  $\sim 1 \mu\text{m}$ .

All data has been recorded using the Lab::Measurement software package [5].

## II. CAPACITIVE SENSITIVITY

The sensitivity of the gate capacitance  $C_g$  on the nanotube position  $z$  depends on several parameters that are experimentally not well-known. In the fit procedure for the results on device A discussed in the main manuscript and below, we have therefore

|                                              | device A            | device B    |
|----------------------------------------------|---------------------|-------------|
| contact metal                                | Re                  | Ti / Pt     |
| contact film thickness                       | 40nm                | 10nm / 40nm |
| distance between the contacts / trench width | 700nm               | 1200nm      |
| initial wafer silicon oxide thickness        | 300nm               | 500nm       |
| etch depth                                   | $\sim 160\text{nm}$ | 100nm       |
| relevant other publications                  | [3]                 | [4]         |

**Supplementary Table S-I.** Fabrication parameters for devices A and B.

---

\* andreas.huettel@ur.de

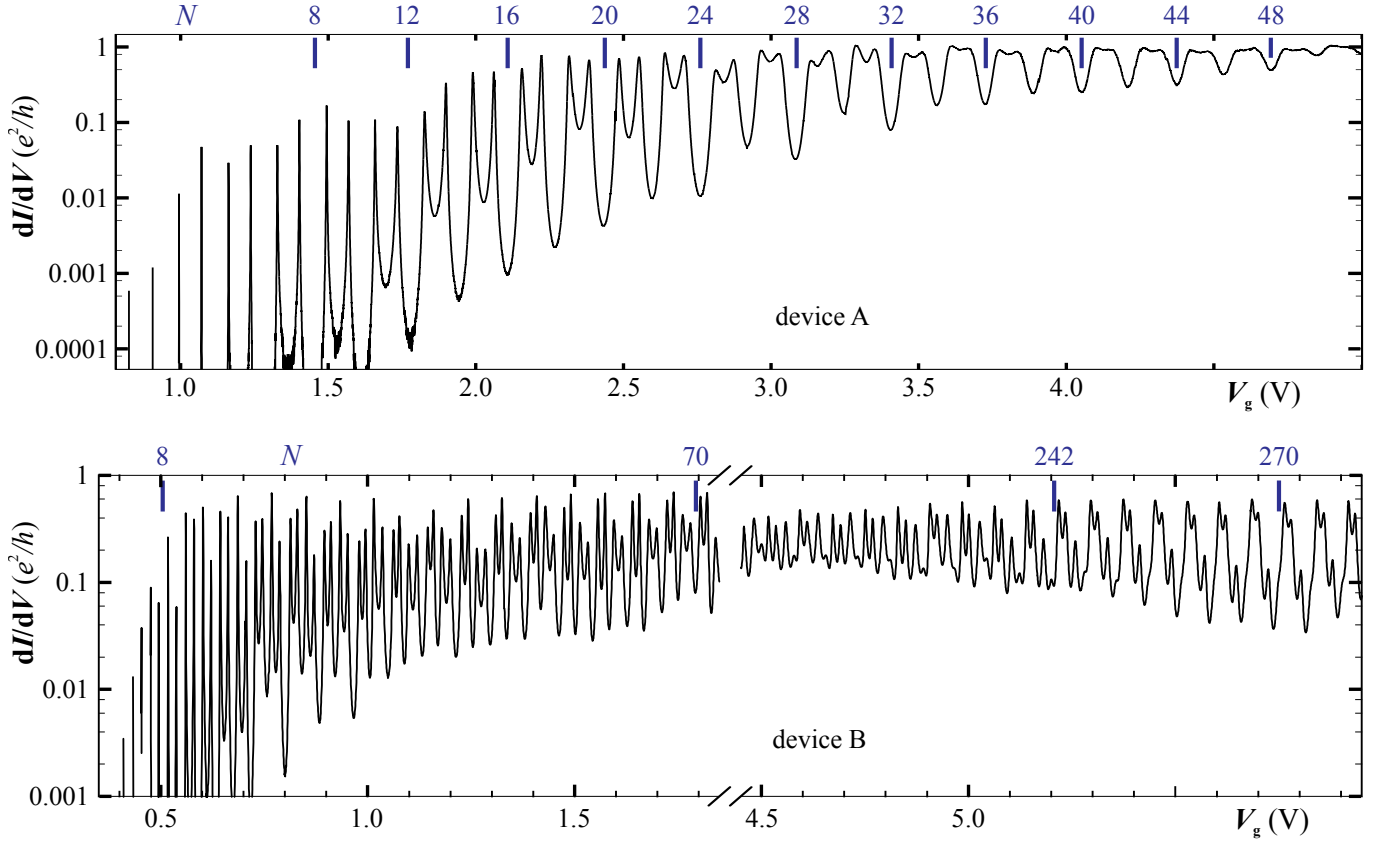

**Supplementary Figure S-1.** Larger version of Fig. 1(b,c) of the main text: low-bias differential conductance  $dI/dV_{sd}$  of carbon nanotube devices A and B as a function of applied back gate voltage  $V_g$ . The number of trapped electrons  $N$  is indicated.

used  $dC_g/dz$  as a free parameter, resulting in

$$\frac{dC_g}{dz} = -27 \frac{zF}{\text{nm}} \quad (\text{S-1})$$

In the following, we estimate this parameter independently and discuss error sources.

A typical simplified model for the gate capacitance of a suspended carbon nanotube is that of a metallic cylindrical beam above a conductive plane,

$$C_g^{\text{th}} = \frac{2\pi\epsilon_0 L}{\ln\left[\frac{2z}{r}\right]} \quad (\text{S-2})$$

where  $L$  is the beam length,  $z$  the distance between beam and plane, and  $r$  is the beam radius. We can estimate the length of our nanotube  $L$  with the distance between the contact electrodes,  $L = 700\text{nm}$ . Since we do in general not image our devices before measurement to avoid contamination, and since this particular device did not survive a subsequent attempt at Raman spectroscopy, we do not know the precise nanotube position or orientation, and larger values are well possible.

The radius of the nanotube is similarly hard to quantify. Measurements of the single electron magnetic moment on the same device result in  $R = 2.2\text{nm}$  [3], though the used model (as published originally in [6]) likely does not capture the entire required physics [3]. The distance between nanotube and gate can be approximated as the sum of gate oxide thickness and contact electrode thickness,  $z = 340\text{nm}$ . This does not take possible slack of the nanotube into account, nor the layer structure of 200nm vacuum (electrode thickness plus etch depth) and 140nm  $\text{SiO}_2$  (remaining oxide) with  $\epsilon_r = 3.9$ . With above approximations, we obtain

$$C_g^{\text{th}} = 6.8\text{aF} \quad (\text{S-3})$$

compared to the value  $C_g = 2.4\text{aF}$  from transport spectroscopy.

The localized electronic system of the quantum dot does not occupy the entire length of the nanotube; we use this to define an electronic length  $L_{\text{el}} < L$  such that the calculated gate capacitance becomes equal the measured one,

$$L_{\text{el}} = \frac{C_g}{C_g^{\text{th}}} L = 250 \text{ nm}. \quad (\text{S-4})$$

Using this length in Eq. S-2 and assuming a uniform deflection along the quantum dot, we obtain at  $z = 340 \text{ nm}$

$$\left. \frac{dC_g}{dz} \right|_{z=340 \text{ nm}} = -1.2 \frac{\text{zF}}{\text{nm}}, \quad (\text{S-5})$$

approximately smaller by a factor 20 than the fit result. A likely conclusion is that our suspended nanotube lies closer to the gate than expected, however, given the many approximations and unknowns no definite statement can be made.

### III. GATE VOLTAGE DEPENDENCE OF THE RESONANCE FREQUENCY

Both for displaying the observed resonance frequency behaviour more clearly and for improving the numerical stability of the fit results, as first step a linear contribution is subtracted from the raw resonance peak positions in Fig. 2(a) of the main text. The resulting resonance frequency shift, converted to angular frequency, is plotted in Figs. 2(d) and 3(a) of the main text (data points):

$$\tilde{\omega}_0(V_g) = 2\pi f_0(V_g) - (a + bV_g), \quad a = 2041 \times 10^6/\text{s}, \quad b = 261.9 \times 10^6/\text{Vs} \quad (\text{S-6})$$

As detailed in [7], the gate voltage dependence of the mechanical resonance frequency in Coulomb blockade consists of essentially three terms:

- a), a continuous increase, corresponding to the continuous increase of the gate charge and the respective tension component,
- b), a step function, corresponding to the stepwise increase of the quantum dot charge and the respective tension component, and
- c), “frequency dips” corresponding to the softening of the spring constant by charge fluctuation whenever single electron tunneling is possible.

Approximating term a) as linear within the evaluated gate voltage region, we obtain as model

$$\omega_0(V_g) = \overbrace{a' + b'V_g}^{\text{a)}} + \overbrace{\kappa \langle N \rangle(V_g)}^{\text{b)}} + \overbrace{\Delta\omega_0(V_g)}^{\text{c)}}. \quad (\text{S-7})$$

As already discussed in the main text, we assume the density of states on the quantum dot to be a sequence of two equal-width Lorentzian peaks, aligned with the Fermi edge of the grounded drain contact at gate voltages  $V_{g1}$  and  $V_{g2}$ , and separated by a corresponding charging energy. Tunnel barrier transparencies for both contacts are equal and energy-independent. In zero temperature approximation, the Fermi distribution in both leads becomes a step function, offset by the small source-drain voltage  $V_{\text{sd}}$ . Following [8], as an example, the tunnel rate into (+) the level corresponding to Coulomb oscillation 1 from the contact L (source) then becomes

$$\Gamma_{1L}^+(V_g) = a \left( \frac{1}{2} + \frac{1}{\pi} \arctan \left( \frac{2e(V_{\text{sd}} + (-V_g + V_{g1})\alpha)}{\Gamma\hbar} \right) \right) \quad (\text{S-8})$$

Writing  $\Gamma_{1/2}^{+/-} = \Gamma_{1/2L}^{+/-} + \Gamma_{1/2R}^{+/-}$  and treating the occupation of the two levels as independent of each other, the time-averaged charge occupation of the quantum dot  $\langle N \rangle(V_g)$  becomes

$$\langle N \rangle(V_g) = N_0 + \frac{\Gamma_1^+}{\Gamma_1^+ + \Gamma_1^-} + \frac{\Gamma_2^+}{\Gamma_2^+ + \Gamma_2^-} \quad (\text{S-9})$$

For the derivation of the frequency “dips”, term c), we then use the expression from [7, 8],

$$\Delta\omega_0 = \frac{V_g(V_g - V_{\text{CNT}})}{2m\omega_0 C_\Sigma} \left( \frac{dC_g}{dz} \right)^2 \left( 1 - \frac{e}{C_g} \frac{\partial \langle N \rangle}{\partial V_g} \right). \quad (\text{S-10})$$

| description                           | parameter  | source             | value                             |
|---------------------------------------|------------|--------------------|-----------------------------------|
| bias voltage                          | $V_{sd}$   | set in measurement | 0.1 mV                            |
| nanotube length                       | $L$        | device geometry    | 700 nm                            |
| nanotube radius                       | $R$        | from [3]           | 2.2 nm                            |
| nanotube mass                         | $m$        | from $L$ and $R$   | 7.4 ag                            |
| gate capacitance                      | $C_g$      | CB evaluation      | 2.4 aF                            |
| total capacitance                     | $C_\Sigma$ | CB evaluation      | 44 aF                             |
| gate lever arm                        | $\alpha$   | CB evaluation      | 0.055                             |
| initial electron number               | $N_0$      | CB evaluation      | 40                                |
| approx. resonance frequency           | $\omega_0$ | Fig. 2             | $3.13 \times 10^9 / \text{s}$     |
| lifetime broadening of levels         | $\Gamma$   | fit result         | $3.41 \times 10^{12} / \text{s}$  |
| constant frequency offset             | $a + a'$   | fit result         | $2.01 \times 10^9 / \text{s}$     |
| linear frequency increase             | $b + b'$   | fit result         | $0.237 \times 10^9 / \text{Vs}$   |
| dot charge-related frequency increase | $\kappa$   | fit result         | $3.07 \times 10^6 / \text{s}$     |
| position CB oscillation 1             | $V_{g1}$   | fit result         | 4.1084 V                          |
| position CB oscillation 2             | $V_{g2}$   | fit result         | 4.1854 V                          |
| capacitive sensitivity                | $dC_g/dz$  | fit result         | $-27 \frac{\text{zF}}{\text{nm}}$ |

**Supplementary Table S-II.** Parameters for Fig. 3 of the main text (device A).

$C_g$  and  $C_\Sigma$  are obtained from Coulomb blockade (CB) measurements;  $m$  is estimated from radius and length of the nanotube (see above).

In a first fitting step the positions of the Coulomb blockade oscillations,  $V_{g1}$  and  $V_{g2}$ , are fixed, and the bare tunnel couplings, the level broadening  $\Gamma$ , the capacitive sensitivity  $dC_g/dz$ ,  $\kappa$ ,  $a'$ , and  $b'$  are used as free parameters. In a subsequent second fitting step, the bare tunnel couplings and the level broadening  $\Gamma$  are fixed and the capacitive sensitivity  $dC_g/dz$ ,  $\kappa$ ,  $a'$ ,  $b'$ ,  $V_{g1}$ , and  $V_{g2}$  are used as free parameters.

The resulting values are summarized in Table **S-II**.

#### IV. COMPARISON WITH GERLAND ET AL. [1]

Figure **S-2** illustrates the analogy between our measurement data, Fig. 3 of the main text, and the results of Gerland *et al.* [1], Fig. 3(c,d) there. The data points and the thick, red solid lines in the three panels display our experimental data and our fit results, respectively, in the same way as Fig. 3 of the main text. The thin black lines in panels (b) and (c) of Fig. **S-2** display the values for the transmission amplitude  $|t(V_g)|$  and the transmission phase  $\phi(V_g)$  extracted from [1], Fig. 3(c,d).

For  $T = 0$  and  $V_{sd} = 0$  Gerland *et al.* calculate  $\langle N_\sigma \rangle$ , where  $\sigma$  indicates the spin, from the Bethe ansatz; using Friedel's sum rule and results from Fermi liquid theory they obtain  $\phi_\sigma = \langle N_\sigma \rangle \pi$  and  $|t_\sigma| = \sin(\phi_\sigma)$ . The result is plotted in Fig. **S-2** for  $\hbar\Gamma = U/25$  (solid),  $\hbar\Gamma = U/4\pi$  (dashed), and  $\hbar\Gamma = U/6$  (dotted). Its  $x$ -axis has been rescaled such that the bare resonance positions ( $-\varepsilon_d/U = 0$  and  $-\varepsilon_d/U = 1$  in [1]) coincide with the bare resonance positions given by our fit, cf. Table **S-II**.

Given that the calculation is for the limit  $T = 0$  and  $V_{sd} = 0$ , we cannot expect perfect agreement. The phase / charge correspondence in Fig. **S-2**(c) indicates that the experiment corresponds to a rather small ratio  $U/\hbar\Gamma$ , with the best correspondence given by the curve for  $U/\hbar\Gamma = 6$  (dotted line). From our experiment and its model fit we obtain  $U_{\text{exp}} = e\alpha(V_{g2} - V_{g1}) = 4.2 \text{ meV}$  and  $\hbar\Gamma = 2.2 \text{ meV}$ , resulting in  $U/\hbar\Gamma = 1.9$ . In the transmission / current correspondence, more distinct differences between the curves occur. Possible origins of these include the finite bias voltage and temperature as well as an experimental situation that goes beyond SU(2) Kondo effect.

Nevertheless, both features discussed in the main text are clearly visible in the experimental data as well as in the calculation from [1]: i), the approximate phase / charge plateau in the gate voltage region of the Kondo conductance ridge, and ii), the distinct “inwards shift” of the large conductance region towards the Kondo ridge center, compared to the bare resonance positions.

---

[1] U. Gerland, J. von Delft, T. A. Costi, and Y. Oreg, “Transmission phase shift of a quantum dot with Kondo correlations,” *Phys. Rev. Lett.* **84**, 3710–3713 (2000).

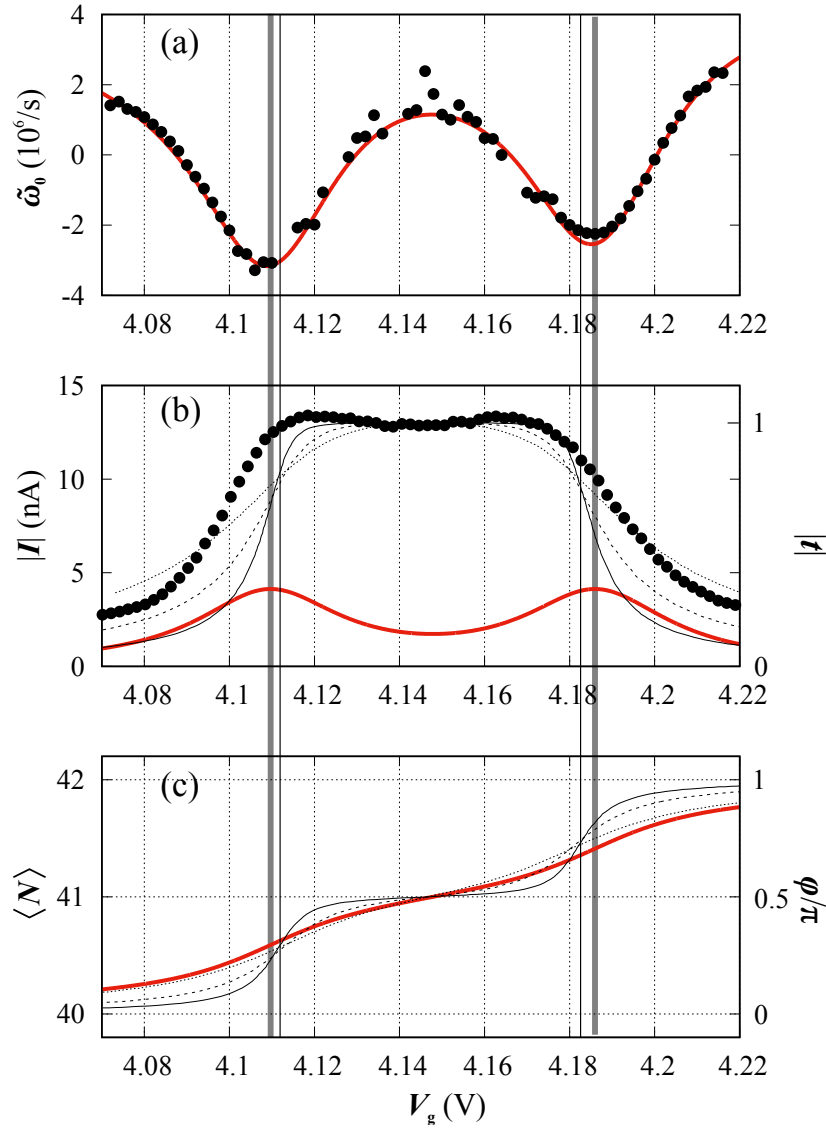

**Supplementary Figure S-2.** Detail comparison of our measurement and our fits with the theoretical results from [1]; extended version of Fig. 3 of the main text. Kondo regime around  $\langle N \rangle = 41$ ;  $V_{sd} = -0.1$  mV. (a) Data points: resonance frequency shift  $\tilde{\omega}_0(V_g)$ . Thick, red solid line: curve fit assuming the subsequent occupation of two non-degenerate levels. (b) Data points: measured off-resonant current  $|I|(V_g)$ . Thick, red solid line: sequential tunneling only current according to the fit model from (a); both left axis. Thin solid, dashed, and dotted black lines: rescaled calculation results from [1], Fig. 3(c), transmission magnitude  $|t|$  through a Kondo resonance for  $T = 0$  and  $\hbar\Gamma = U/25, U/4\pi, U/6$ ; right axis. (c) Thick, red solid line: time-averaged quantum dot occupation  $\langle N \rangle(V_g)$  derived from the fit in (a); left axis. Thin solid, dashed, and dotted black lines: rescaled calculation results from [1], Fig. 3(d), for the transmission phase  $\phi$ ;  $\hbar\Gamma = U/25, U/4\pi, U/6$ ; right axis. Thick vertical lines: bare resonance positions, thin vertical lines: approximate locations of maximal slope of  $\phi(V_g)$ .

- [2] J. Kong, H. T. Soh, A. M. Cassell, C. F. Quate, and H. Dai, "Synthesis of individual single-walled carbon nanotubes on patterned silicon wafers," *Nature* **395**, 878 (1998).
- [3] M. Marganska, D. R. Schmid, P. L. Stiller, A. Dirnauichner, Ch. Strunk, M. Grifoni, and A. K. Hüttel, "Shaping electron wave functions in a carbon nanotube with a parallel magnetic field," (2017), arXiv:1712.08545.
- [4] A. Dirnauichner, M. del Valle, K. J. G. Götz, F. J. Schupp, N. Paradiso, M. Grifoni, Ch. Strunk, and A. K. Hüttel, "Secondary electron interference from trigonal warping in clean carbon nanotubes," *Physical Review Letters* **117**, 166804 (2016).
- [5] S. Reinhardt, C. Butschkow, S. Geissler, A. Dirnauichner, F. Olbrich, C. Lane, D. Schröer, and A. K. Hüttel, "Lab::Measurement — a portable and extensible framework for controlling lab equipment and conducting measurements," (2018), arXiv:1804.03321.
- [6] E. D. Minot, Yuval Yaish, Vera Sazonova, and Paul L. McEuen, "Determination of electron orbital magnetic moments in carbon nanotubes," *Nature* **428**, 536 (2004).
- [7] G. A. Steele, A. K. Hüttel, B. Witkamp, M. Poot, H. B. Meerwaldt, L. P. Kouwenhoven, and H. S. J. van der Zant, "Strong coupling between single-electron tunneling and nanomechanical motion," *Science* **325**, 1103 (2009).

- [8] H. B. Meerwaldt, G. Labadze, B. H. Schneider, A. Taspinar, Y. M. Blanter, H. S. J. van der Zant, and G. A. Steele, “Probing the charge of a quantum dot with a nanomechanical resonator,” *Phys. Rev. B* **86**, 115454 (2012).
